# Supplementary material for: Evaluating the impact of incomplete contact tracing data on urban epidemic dynamics
Source: arXiv:2601.14632 ancillary file (2026-08-15)
Supplement: Supplementary file 1 [file CT_ABM_supplementary.pdf]

# Supplementary Information

## Contents

**S1 Agent characteristics in the synthetic population** **2**
S1.1 Household . . . 3
S1.2 Regional residence . . . 3
S1.3 Age . . . 3
S1.4 School classroom . . . 3
S1.5 Workplace . . . 4
S1.6 Friendship . . . 4
S1.7 Comparison of commuting patterns in virtual Seoul and Busan . . . 5

**S2 Contact types and daily routines in the ABM model** **5**

**S3 Contact duration time per each location** **6**

**S4 Simulation results** **7**
S4.1 Results in virtual Seoul . . . 7
S4.2 Results in virtual Busan . . . 7

# S1 Agent characteristics in the synthetic population

The section describes a synthetic population used in the agent-based model (ABM). The synthetic population replicates the demographic structure of Seoul (Busan) by incorporating various public statistical datasets. To construct the synthetic population, we utilize the 2020 2% census data of Seoul (Busan) from the MicroData Integrated Service [S1]. This dataset contains records for 145,817 (61,217) individuals across 66,243 (27,602) households, offering information such as household ID, regional residence, and age. The data spans 25 (16) distinct administrative 2-level region.

To generate a full-scale synthetic population that aligns numerically with both household- and individual-level constraints, we apply the iterative proportional updating algorithm [S2]. The method expands the 2% sample to 100% population. Constraints are imposed at two levels: at the household-level, by the distribution of household counts by region and household size; and at the individual-level, by population counts stratified by region and age group. These constraint values are based on public statistics provided by the Korean Statistical Information Service [S3, S4].

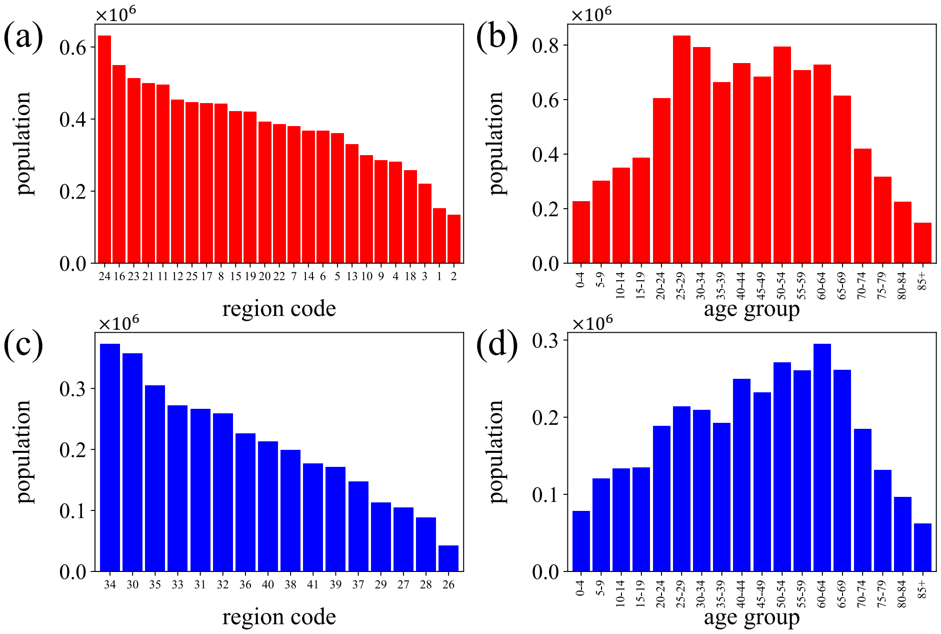


Figure S1: Region and age group histograms of the synthetic population we generated (a, b) in virtual Seoul and (c, d) in virtual Busan. The synthetic population is constructed using the 2% census and expanded to 100% via iterative proportional updating algorithm to numerically match public population statistics. The distributions closely replicate real-world demographic structures.

As a result, the synthetic population of Seoul comprises 9,529,266 agents distributed across 4,289,230 households. These synthetic values closely approximate Seoul's actual population statistics, which report 9,384,512 individuals and 4,141,659 households. Similarly, the synthetic population of Busan consists of 3,313,542 agents across 1,498,812 households, closely matching the actual structures of 3,279,604 individuals and 1,462,404 households. To ensure that the synthetic populations replicate real-world demographic structures, we examined the age group and region histograms of agents in virtual Seoul and virtual Busan (see, Figure S1)

In this model, each agent in the synthetic population is assigned sociodemographic attributes to simulate daily behavior. These attributes are used to construct a realistic representation of virtual Seoul (the same method is applied for virtual Busan). The model includes six characteristics: household ID, residence, age, educational status, economic activity, and friendship network (see, Figure S2). For example, index 1 represents an agent assigned to household ID 1564065, living in region 12, aged 1 year, with no educational or economic activity, and connected to 10 friends. Index 1 and index 2 are household members residing in the same household. Index 2 and index 3 are coworkers at the same workplace. While index 3 resides in the same region as their workplace, index 2 commutes from a different region. Index 4 and index 5 are classmates, and index 5 has a long commuting distance. Index 6 is the teacher assigned to both index 4 and index 5.

| index | agent ID | household ID | residence | age | edu region | classroom ID | eco region | workplace ID | # of friends | friend's list |
|---|---|---|---|---|---|---|---|---|---|---|
| 1 | 3461258 | 1564065 | 12 | 1 | 0 | 0 | 0 | 0 | 10 | [2135687, 2245225, …] |
| 2 | 3461259 | 1564065 | 12 | 33 | 0 | 0 | 13 | 302903 | 32 | [621119, 653133, …] |
| 3 | 3541682 | 1601851 | 13 | 44 | 0 | 0 | 13 | 302903 | 22 | [77722, 847097, …] |
| 4 | 5501151 | 2470724 | 1 | 17 | 1 | 11006 | 0 | 0 | 40 | [1146105, 5505787, …] |
| 5 | 4575752 | 2069222 | 8 | 17 | 7 | 11006 | 0 | 0 | 22 | [88722, 847097, …] |
| 6 | 6200063 | 3087749 | 20 | 45 | 0 | 11006 | 1 | 0 | 12 | [816881, 1331729, …] |
| 7 | 4575752 | 2069222 | 24 | 83 | 0 | 0 | 0 | 0 | 84 | [8938339, 847097, …] |
| 8 | 8938339 | 4039913 | 24 | 80 | 0 | 0 | 0 | 0 | 13 | [4575752, 309503, …] |
| 9 | 3201786 | 1450478 | 11 | 59 | 0 | 0 | 11 | 259651 | 11 | [1260714, 2964441, …] |
| 10 | 1817128 | 848395 | 5 | 51 | 0 | 0 | 0 | 0 | 52 | [1260714, 6672841, …] |

Figure S2: Partial example of the synthetic population structure. The table illustrates the relationships between agents based on household, classroom, workplace, and friendship networks. Index 1 and 2 belong to the same household; index 2 and 3 share a workplace; index 4 and 5 are classmates; index 6 is the teacher of index 4 and 5; index 7 and 8 are friends; and index 9 and 10 are connected via a mutual friend (agent ID 1260714).

Index 7 and index 8 are friends. Index 9 and index 10 share a common friend (agent ID 1260714).

Among these, household ID, residence, and age are not assigned arbitrarily but are directly derived from the census data. These attributes are expanded proportionally to create a full-scale population, preserving their distribution. Household IDs are re-assigned during this expansion to ensure unique household identification. The remaining characteristics-education, economy, and friendship-are generated using national-level statistical sources such as enrollment rates, employment data, and etc.

## S1.1 Household

The household refers to a residential unit, and each agent is assigned to exactly one household. Each household is uniquely identified by a household ID, and no agent belongs to more than one household.

## S1.2 Regional residence

Each agent is assigned a residential region represented by a region code (number). Seoul comprises 25 districts, and Busan consists of 16 districts. All members of the same household have the same residence number. For students and office workers, additional region information is included to indicate the district of their assigned classroom or workplace, which may differ from their region of residence.

## S1.3 Age

Each agent is assigned an integer age ranging from 0 to 85. Since the census data provides age only up to 85, all individuals aged above 85 in the real population are modeled as 85 years old.

## S1.4 School classroom

The synthetic population includes information on agents' educational status, specifying whether they are currently affiliated with an educational institution. Those who are enrolled or employed at such institutions are categorized as students or teachers, respectively. Their educational attribute includes the identifier of the classroom to which they are assigned. Students are between the ages of 3 and 18, while teachers range in age from 19 to 84.

We calculated the number of students according to the region-based enrollment rate by age group and randomly selected agents to become students [S2, S5, S6, S7, S8]. They have the classroom ID they belong to as education information. The ages of agents belonging to the same classroom are the same. Since there is no concept of "school" in the model, there is no connection between classrooms. The average number of students in each classroom was calculated using actual data on the number of students per class in Seoul (Busan).

In addition, education also includes spatial information. The location of the classroom is indicated as a district like a residence. Using the age-specific regional day and night resident population data created using the Korea Telecom DataBase, we created students who commute to other regions than their residence. In other words, the education information includes information on the classroom ID they belong to and the district where the classroom is located.

### S1.5 Workplace

The synthetic population also includes economic activity status, indicating whether an individual is the economically active population. Only agents aged between 19 and 84 are considered eligible for economic activity. Similar to students, economically active agents may commute to a different region than where they reside. This commuting pattern is reflected in the economic attribute, which records the agent's workplace location. Economically active agents are categorized into two types: office workers and teachers. Office workers are assigned a workplace ID, while teachers are associated with a classroom ID.

We calculated the number of economically active agents in each region based on the employment rate data by age group and region [S9], and selected agents who would become office workers (teachers) [S2]. They have the workplace ID (classroom ID) to which they belong as economy (education) information. The size of the workplace is small and large, with an average of 5 and 10, respectively, and the ratio was calculated using actual data on the number of companies in Seoul (Busan) [S10]. The number of teachers in each classroom was calculated using actual data on the number of teachers per student in Seoul (Busan) [S5, S6, S7, S8]. Thus, teachers were assigned according to the number of students in each classroom.

### S1.6 Friendship

The synthetic population incorporates friendship networks, where each agent is associated with a list of friends represented by their agent IDs. The agent ID corresponds to the index number assigned to an agent. Friendships are modeled as mutual connections-if agent $A$ includes agent $B$ in their friend list, then agent $B$ likewise includes agent $A$ in theirs. Friend lists are constructed using a homophilic Barabási-Albert (BA) network model [S11], where age serves as the homophily attribute and all links are bidirectional.

In Korean society, age strongly influences social relationships, including how friendship is defined. Because of age-based hierarchies rooted in Confucian traditions, people are typically considered "friends" only if they are the same age, while age differences tend to create hierarchical relationships [S12, S13]. This is particularly evident in friendship formation, where individuals tend to associate with peers of similar age due to cultural norms surrounding honorific speech, seniority, and shared life-stage experiences. Such age-based affinity is deeply embedded in everyday interactions and is often more salient than other sociodemographic factors. To capture this cultural feature, we implemented a homophilic mechanism in the construction of the friendship network, where agents are more likely to form connections within the same 10-year age group. The homophily parameter was set to 0.9 to reflect the strong age-based clustering observed in real-world Korean social networks.

Two separate procedures are used to generate (1) local friendships and (2) cross-regional friendships. In both cases, agents are randomly sampled in groups of 1,000 agents who belong to the same age group, defined by 10-year intervals. For local friendships, all selected agents must reside in the same administrative region, whereas for cross-regional friendships, residence is not restricted-agents can form connections with others from different regions.

Each group of 1,000 agents is used to grow a homophily BA network. Once a connection is formed, the linked agents record each other's agent ID in their respective friend lists. Specifically, the homophilic BA model begins with an initial ring of 10 agents. Each newly added agent creates 5 connections to existing nodes, with attachment probability weighted both by the degree of existing nodes and by age match. The age match is implemented as a binary condition within the same 10-year age group, and the homophily strength is controlled by a parameter $h = 0.9$, which linearly increases the likelihood of forming connections with agents from the same age group (10 yr). This approach embeds demographic realism into the synthetic social network, particularly in the Korean context where age hierarchy significantly influences peer relationships.

In the resulting synthetic population, the average number of friends per agent is 20, with a standard deviation of 13. The most connected agent has 228 friends, while the least connected has 7.

### S1.7 Comparison of commuting patterns in virtual Seoul and Busan

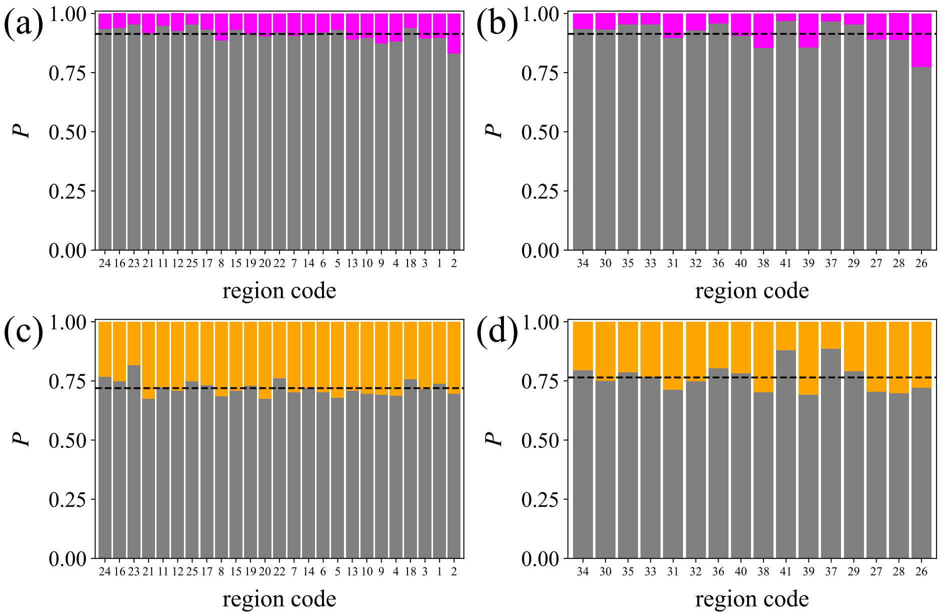


Figure S3: Long- and short-distance commuting patterns by region for (a-b) students (top panel) and (c-d) office workers (bottom panel) in the synthetic populations of (a, c) virtual Seoul, and (b, d) virtual Busan. Grey bars indicate the proportion of agents whose residence and school classroom/workplace are in the same administrative region, while colored bars indicate those who commute to different regions. The horizontal dashed lines represent the average proportions.

Long-distance commuters are defined as agents whose schools or workplaces are located in administrative districts different from their residential region. Figure S3 shows the proportion of long- and short-distance commuters among students and office workers (teachers) in the synthetic populations. Long-distance commuters are agents whose school classrooms (workplaces) are located in different regions from their residence, while short-distance commuters remain within their residence. In virtual Seoul, the proportion of long-distance student commuters is 8.64%, and that of workers is 28.05% (see, Figure S3(a, d)). In virtual Busan, the rate for students is similar (8.62%), but for office workers, it is lower at 23.54%, approximately 5% below Seoul (see, Figure S3(b, e)).

## S2 Contact types and daily routines in the ABM model

Table S1: Summary of contact types in the simulation.

| contact type | frequency | size (average) |
|---|---|---|
| household | daily | size of each household |
| school classroom | weekdays | 6–45 (21.3) |
| workplace | weekdays | 1–39 (5.9) |
| friends' gathering | 1/7 | 2–20 (3.2) |
| random encounter | 1/7 | 2–12 (6.0) |

The simulation models each agent's daily routine based on their sociodemographic attributes within the synthetic population. The agents can engage in five types of social contact: household, school classroom, workplace, friends' gatherings, and random encounters within the local community. Among these, household,

classroom, and workplace interactions occur on a regular basis-household contact happens daily, while school classrooms and workplaces are only active on weekdays (see, Table. S1).

In contrast, friends' gatherings and random encounters are modeled as non-routine interactions. These two forms differ in nature: friends' gatherings involve interactions among agents listed as friends, whereas random encounters represent incidental interactions with unknown agents in shared community spaces. To replicate friends' gatherings, each agent is assigned a predefined list of friends, and the decision to meet them is made daily with a probability of 1/7. Because the participants of a gathering are selected from each agent's friend lists, it is also possible for an agent to meet a friend of a friend. The size of such gatherings ranges between 2 and 20 participants.

Random encounters are treated as spontaneous social interactions.Therefore, agents interact with randomly selected agents from the entire population, who may or may not be part of their existing social networks. Each agent has a 1/7 probability of engaging in such interactions on any given day, during which they are expected to come into contact with an average of 5 other agents.

## S3 Contact duration time per each location

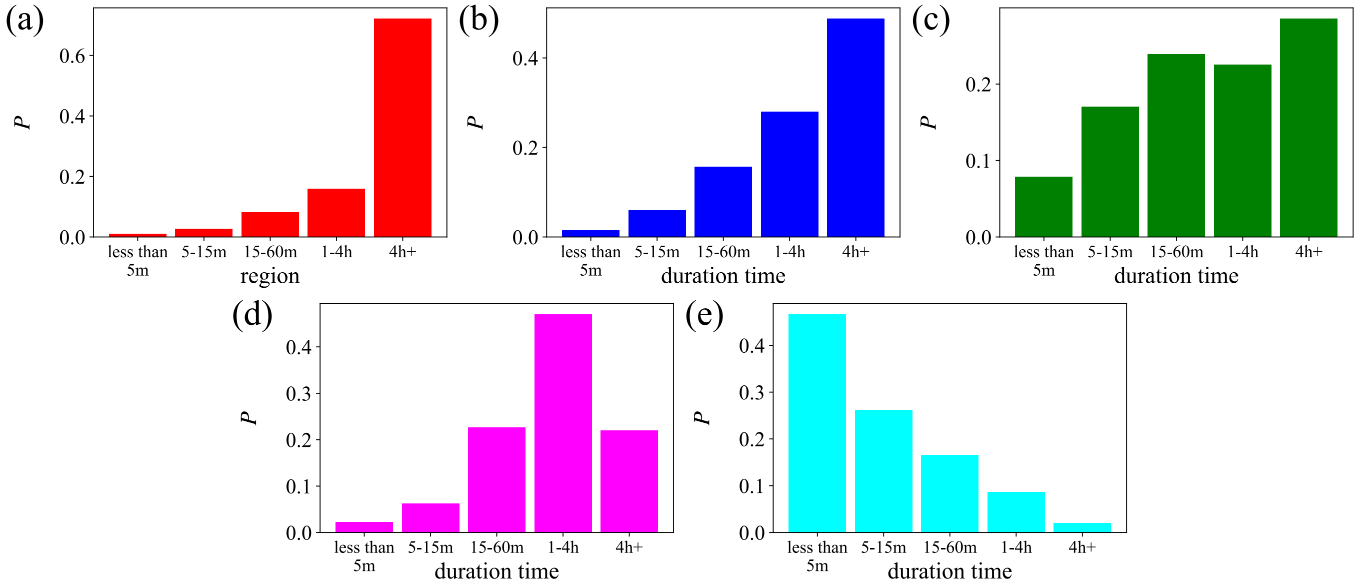


Figure S4: Distribution of contact duration ($t_n$) by location (layer): (a) household, (b) classroom, (c) workplace, (d) friends' gathering, and (e) local community. The top represents regular (routine) contacts, while the bottom corresponds to non-routine contacts.

In this model, infections spread according to a duration-based transmission probability. The transmission equation is defined as $P_{ij} = 1 - e^{-\lambda_{ij}}$ where $\lambda_{ij} = B_n t_n^{ij} \varphi_j$ in the model. In this equation, $t_n^{ij}$ denotes the duration of contact between agent $i$ and agent $j$ at location $n$.

Here, $t_n^{ij}$ represents the contact time between agents $i$ and $j$ at location $n$. Figure S4 presents the distribution of contact durations ($t_n$) by location type, based on a large-scale close-contact survey conducted in South Korea during 2023–24 [S14]. In the survey, contact duration was recorded using categorical (multiple-choice) responses rather than exact time values. For each agent, the contact duration ($t_d$) by location is assigned using the corresponding the distributions as a weight. Then, the actual duration in minutes is randomly drawn from a uniform random number generator within the selected time range.

For example, if two agents contact in the household, the duration category is selected using the weighted distribution shown in Figure S4(a). If the selected category is "$4h+$", the actual contact time is drawn uniformly between 240 and 720 minutes, assuming a maximum contact duration of 12 hours.

## S4 Simulation results

In our study, we did not have access to real-world contact tracing records for direct validation. Therefore, we conduct validation to enhance the credibility of our simulation results.

We compared outcomes by doubling the number of initial infected agentsm and then examined results across two cities—Seoul and Busan—that differ significantly in population size.

### S4.1 Results in virtual Seoul

The following results represent the simulated outbreak of a emerging infectious disease in virtual Seoul under the implementation of the CT policy.

Figure S5 presents the results of (Scenario 1) infector-omission, (Scenario 2-1) selective contact-omission, and (Scenario 2-2) uniform contact-omission. In each figure, the left panel corresponds to simulations with 20 initial $E$ agents, while the right panel shows results with 40 initial $E$ agents.

### S4.2 Results in virtual Busan

The following results illustrate the simulated outbreak of a emerging infectious disease in virtual Busan under the implementation of the CT policy.

Figure S5 presents the results of (Scenario 1) infector-omission, (Scenario 2-1) selective contact-omission, and (Scenario 2-2) uniform contact-omission. In each figure, the left panel corresponds to simulations with 20 initial $E$ agents, while the right panel shows results with 40 initial $E$ agents.

# References


[S1] MDIS. 2% census in south korea (korean). *statistics* `https://mdis.kostat.go.kr/eng/index.do`, 2020.

[S2] Min-Kyung Chae, Dong-Uk Hwang, Kyeongah Nah, and Woo-Sik Son. Evaluation of covid-19 intervention policies in south korea using the stochastic individual-based model. *Scientific Reports*, 13(1):18945, 2023.

[S3] KOSIS. Number of household by a household size (korean). *statistics* `https://kosis.kr/statHtml/statHtml.do?orgId=101&tblId=DT_1JC1502&conn_path=I2`, 2023.

[S4] KOSIS. Number of individuals by region and age group (korean). *statistics* `https://kosis.kr/statHtml/statHtml.do?orgId=101&tblId=DT_1IN1503&conn_path=I2`, 2023.

[S5] KOSIS. Kindergarten overview (korean). *statistics* `https://kosis.kr/statHtml/statHtml.do?orgId=334&tblId=DT_1963003_001&conn_path=I2`, 2023.

[S6] KOSIS. Elementary school overview (korean). *statistics* `https://kosis.kr/statHtml/statHtml.do?orgId=334&tblId=DT_1963003_002&conn_path=I2`, 2023.

[S7] KOSIS. Junior school overview (korean). *statistics* `https://kosis.kr/statHtml/statHtml.do?orgId=334&tblId=DT_1963003_003&conn_path=I2`, 2023.

[S8] High school overview (korean). *statistics* `https://kosis.kr/statHtml/statHtml.do?orgId=334&tblId=DT_1963003_004&conn_path=I2`, 2023.

[S9] KOSIS. Working-age population by age (korean). *statistics* `https://kosis.kr/statHtml/statHtml.do?orgId=101&tblId=DT_1DA7015S&conn_path=I2`, 2023.

[S10] KOSIS. Number of businesses by employee size. *statistics* `https://kosis.kr/statHtml/statHtml.do?orgId=101&tblId=DT_1K52D03&conn_path=I2`, 2022.

[S11] Eun Lee, Fariba Karimi, Claudia Wagner, Hang-Hyun Jo, Markus Strohmaier, and Mirta Galesic. Homophily and minority-group size explain perception biases in social networks. *Nature human behaviour*, 3(10):1078–1087, 2019.

[S12] Young Joon Choi, Hyun Jin Kim, and Sung Ho Lee. Cultural values underlying age-based hierarchy and respect for elders in korea. *Journal of Cross-Cultural Gerontology*, 34(3):247–263, 2019.

[S13] Postechian Column. Age hierarchy and the meaning of friendship in korean society, 2023. Accessed: 2025-12-16.

[S14] Woo-Sik Son, Min-Kyung Chae, Dong-Uk Hwang, Kyeongah Nah, Minsoo Kim, Jong-Hoon Kim, and Jonggul Lee. Social contact patterns in south korea: an analysis of a survey conducted in 2023-2024. *BMC Infectious Diseases*, 25(1):295, 2025.

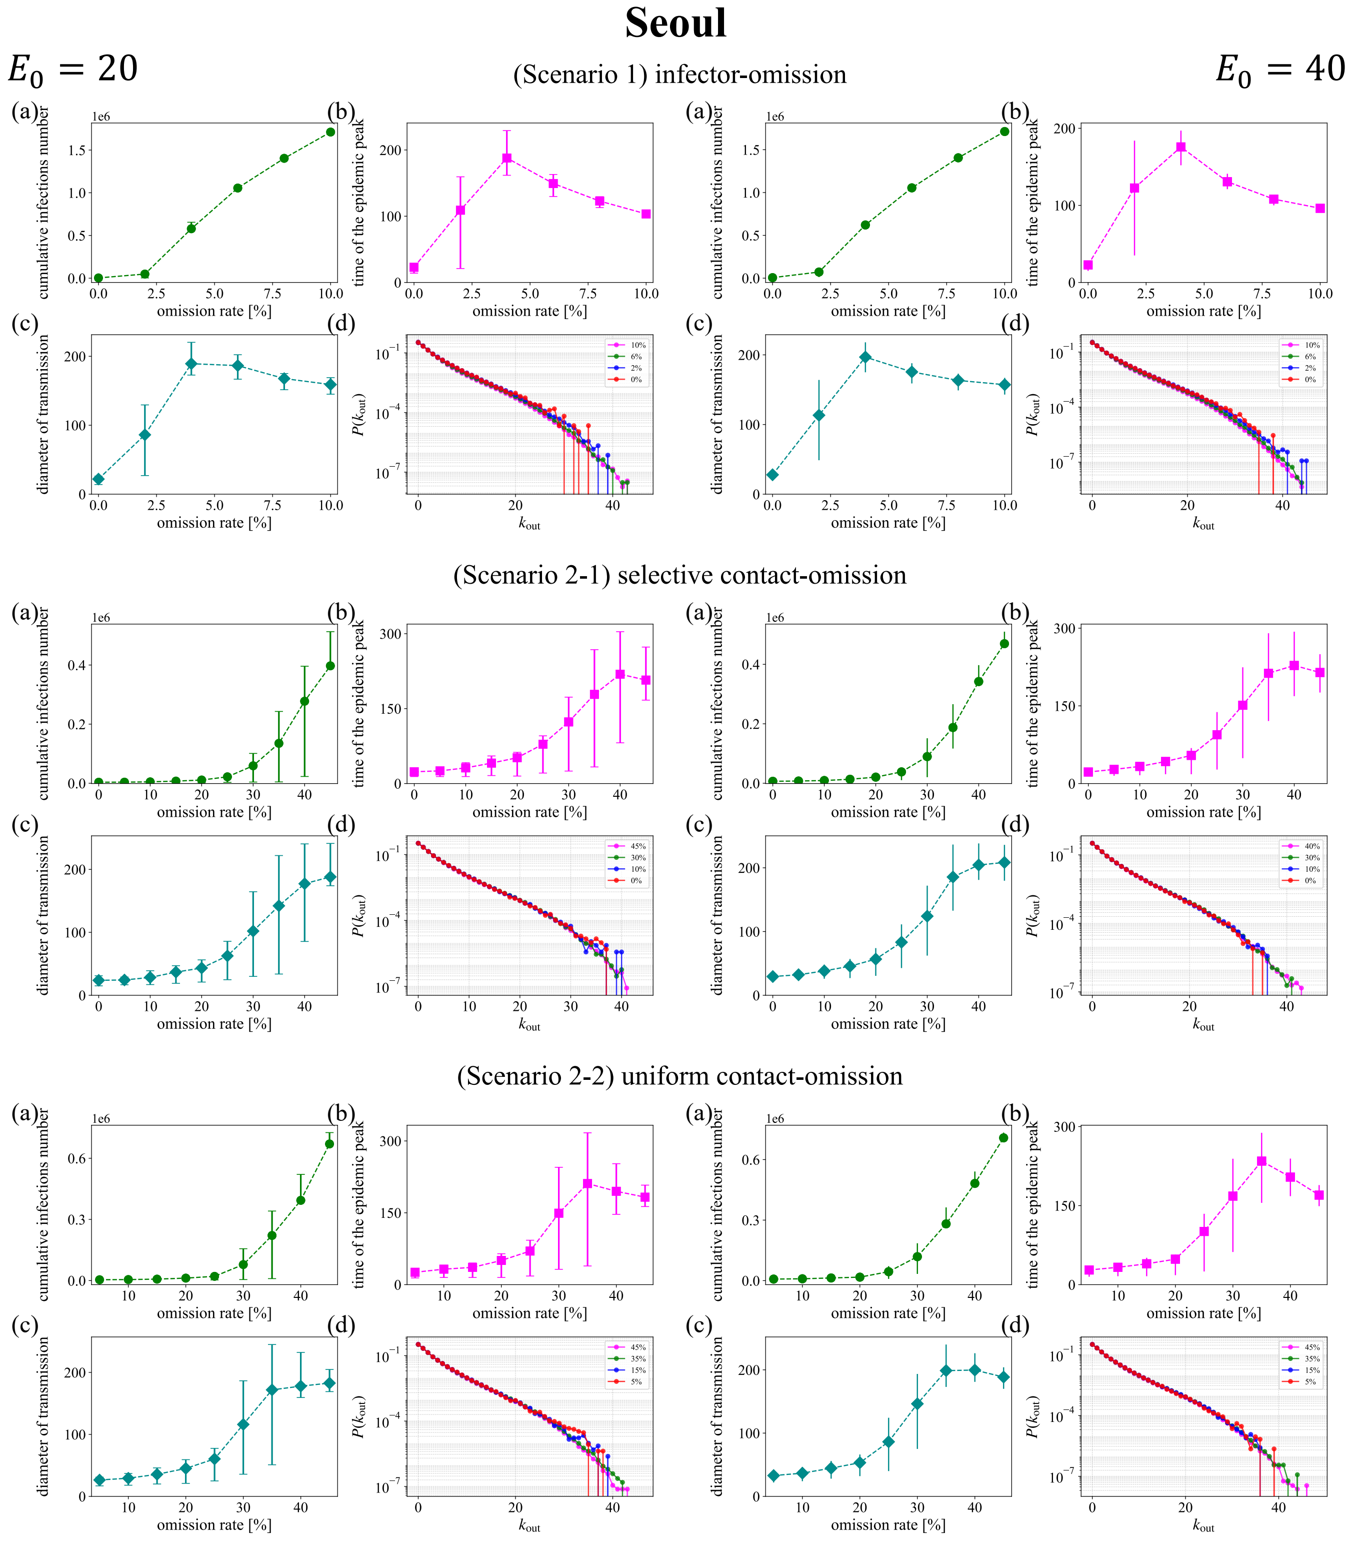


Figure S5: Simulation results for virtual Seoul under different omission scenarios and initial infection sizes. Panels (a–d) show results with 20 initial $E$ agents, and panels (a′–d′) with 40 initial $E$ agents. For each scenario, we report (a, a′) the mean cumulative number of infections, (b, b′) the mean time of the epidemic peak, (c, c′) the mean diameter of the directed transmission network, and (d, d′) the out-degree distribution of the directed transmission network (with the log-scale vertical axis). Results are compared between infector-omission and selective contact-omission (omission in friends' gathering/community layers) and uniform contact-omission (omission across all layers).

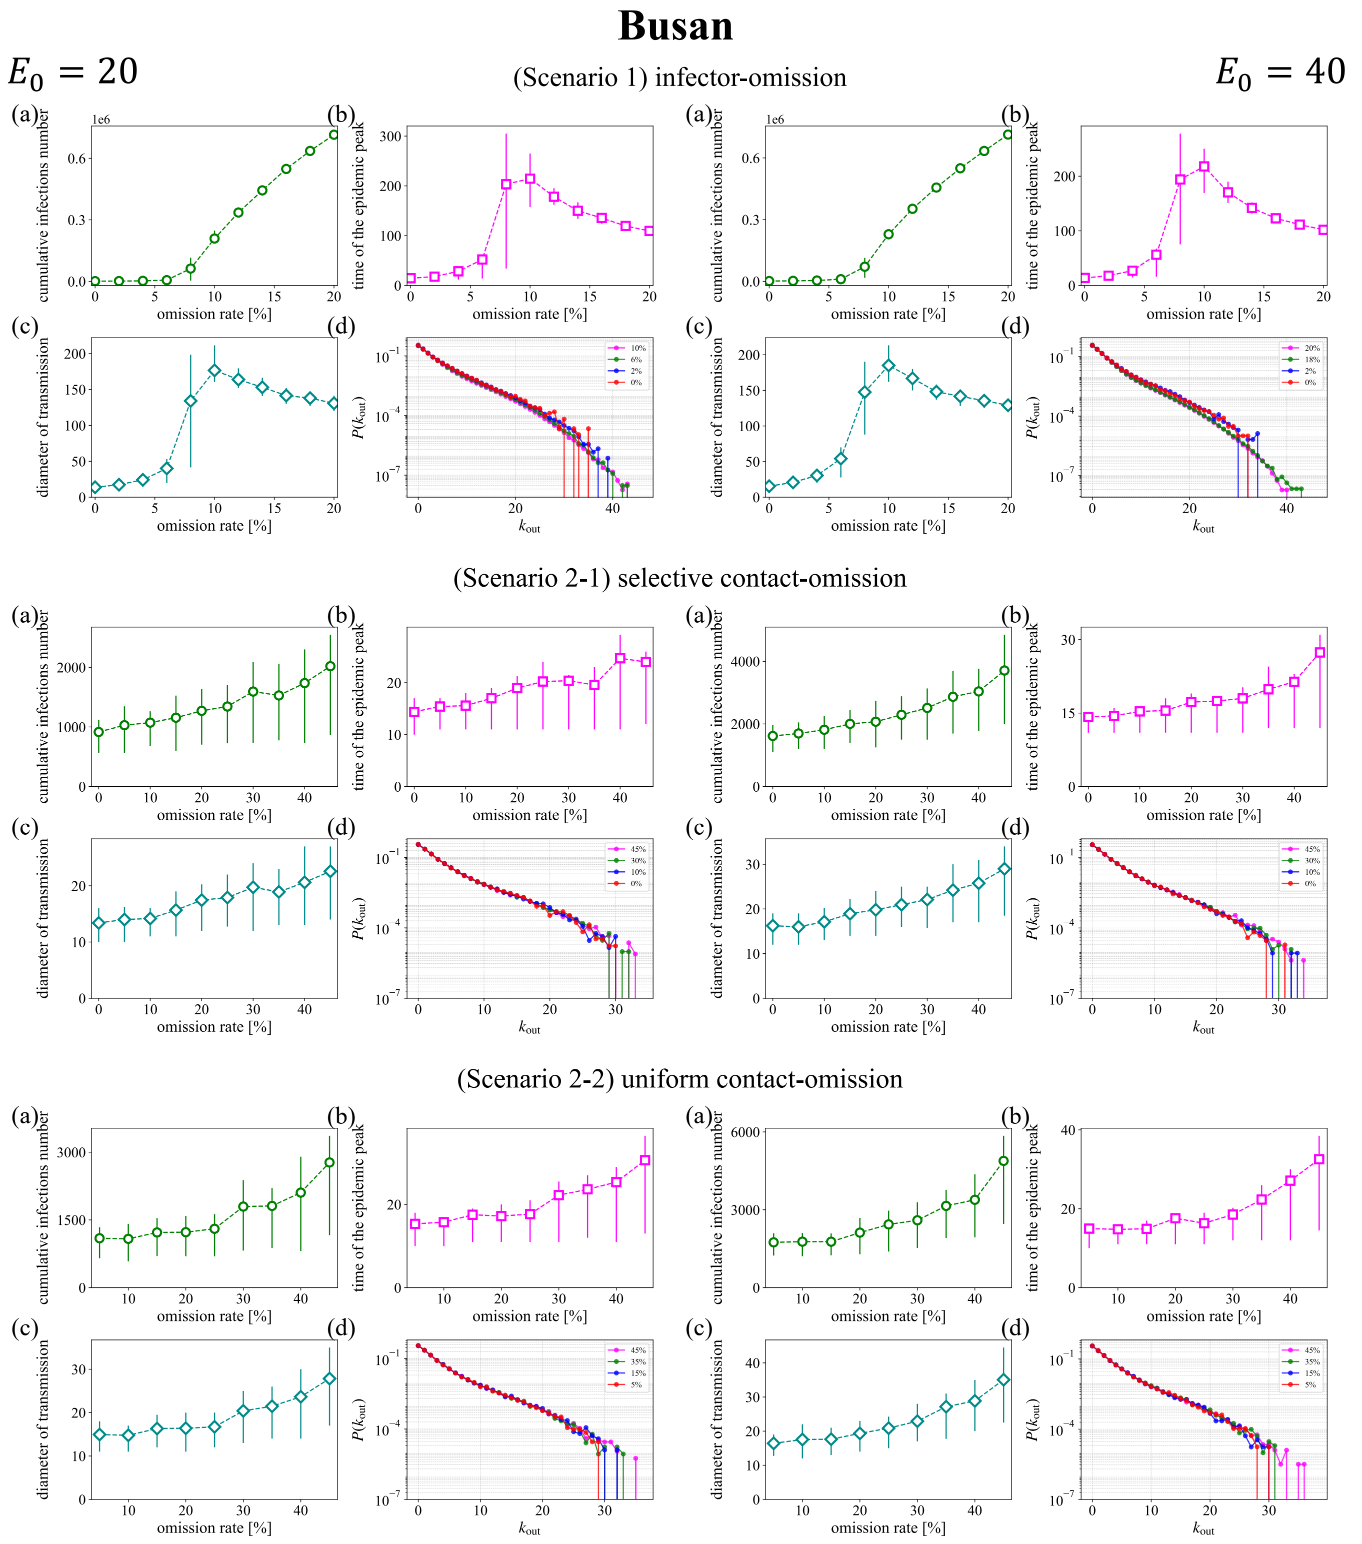


Figure S6: Simulation results for virtual Busan under different omission scenarios and initial infection sizes. Panels (a–d) show results with 20 initial $E$ agents, and panels (a′–d′) with 40 initial $E$ agents. For each scenario, we report (a, a′) the mean cumulative number of infections, (b, b′) the mean time of the epidemic peak, (c, c′) the mean diameter of the directed transmission network, and (d, d′) the out-degree distribution of the directed transmission network (with the log-scale vertical axis). Results are compared between infector-omission and selective contact-omission (omission in friends' gathering/community layers) and uniform contact-omission (omission across all layers).
